# Supplementary material for: signSGD: Compressed Optimisation for Non-Convex Problems
Source: arXiv:1802.04434 source file (2018-08-07)
Supplement: Supplementary file 1 [file small-batch.tex]

\section{Small batch \signSGD{} theory}
\label{app:small}

\textbf{Disclaimer:} this section was developed after the paper was accepted, and has not been through peer review. We include it for completeness.

Theorems \ref{thm:signSGD}, \ref{thm:majority} and \ref{thm:signum} all make use of a batch size as large as the total number of iterations $K$. This means that the total number of gradient calls, $N$, after $K$ iterations satisfies $N = O(K^2)$. As mentioned in Appendix \ref{app:sgdtheory}, large batch algorithms are theoretically preferred to small batch algorithms due to their systems benefits. Specifically, fewer iterations are required for convergence, meaning a smaller wall-clock time for training (assuming the large batch can be parallelised). For \SGD{}, this has been borne out in practice \cite{Goyal2017AccurateLM}.

Despite the systems benefits of large batch training for large scale problems, small batch training is still common since the extra noise is believed to be good for generalisation \cite{smithbayes}. Indeed the experiments in this paper were conducted at a maximum batch size of 256. Therefore a small batch theory for \signSGD{} is desired.

To build such a theory, we must introduce an additional assumption of unimodal symmetric gradient noise. As mentioned in Section \ref{sec:majority} of the main text, this assumption is reasonable in practice even for a modest mini-batch size due to the central limit theorem. We validate the assumption empirically in Figure \ref{fig:symmetry}. Without this assumption, the failure probability of a sign bit can be larger than $\frac{1}{2}$, as mentioned at the end of Section \ref{sec:majority}, and this can prevent convergence.

\begin{lemma}[Failure probability of a sign bit under conditions of unimodal symmetric gradient noise]\label{lem:symm}

Let $\tilde{g}_i$ be an unbiased stochastic approximation to gradient component $g_i$, with variance bounded by $\sigma_i^2$. Further assume that the noise distribution is unimodal and symmetric. Define signal-to-noise ratio $S_i:= \frac{|g_i|}{\sigma_i}$. Then we have that
\begin{align*}
\mathbb{P}[\text{sign}(\tilde{g}_i)\neq\text{sign}(g_i)] 
&\leq \begin{cases}
\frac{2}{9}\frac{1}{S_i^2} & \quad \text{if } S_i > \frac{2}{\sqrt{3}},\\
\frac{1}{2}-\frac{S_i}{2\sqrt{3}} & \quad \text{otherwise}
\end{cases}
\end{align*}
which is in all cases less than $\frac{1}{2}$.
\end{lemma}
\begin{proof}
Recall Gauss' inequality for unimodal random variable X with mode $\nu$ and expected squared deviation from the mode $\tau^2$ \cite{gauss,threesigma}:
\begin{equation*}
\mathbb{P}[|X-\nu| > k] \leq \begin{cases}
\frac{4}{9}\frac{\tau^2}{k^2} & \quad \text{if } \frac{k}{\tau}> \frac{2}{\sqrt{3}},\\
1-\frac{k}{\sqrt{3}\tau} & \quad \text{otherwise}
\end{cases}
\end{equation*}
By the symmetry assumption, the mode is equal to the mean, so we replace mean $\mu = \nu$ and variance $\sigma^2 = \tau^2$.
\begin{equation*}
\mathbb{P}[|X-\mu| > k] \leq \begin{cases}
\frac{4}{9}\frac{\sigma^2}{k^2} & \quad \text{if } \frac{k}{\sigma}> \frac{2}{\sqrt{3}},\\
1-\frac{k}{\sqrt{3}\sigma} & \quad \text{otherwise}
\end{cases}
\end{equation*}
Without loss of generality assume that $g_i$ is negative. Then applying symmetry followed by Gauss, the failure probability for the sign bit satisfies:
\begin{align*}
\mathbb{P}[\text{sign}(\tilde{g}_i)\neq\text{sign}(g_i)] &= \mathbb{P}[\tilde{g}_i - g_i\geq|g_i|] \\
&=\frac{1}{2}\mathbb{P}[|\tilde{g}_i - g_i|\geq|g_i|] \\
&\leq \begin{cases}
\frac{2}{9}\frac{\sigma_i^2}{g_i^2} & \quad \text{if } \frac{|g_i|}{\sigma}> \frac{2}{\sqrt{3}},\\
\frac{1}{2}-\frac{|g_i|}{2\sqrt{3}\sigma_i} & \quad \text{otherwise}
\end{cases}\\
&= \begin{cases}
\frac{2}{9}\frac{1}{S_i^2} & \quad \text{if } S_i > \frac{2}{\sqrt{3}},\\
\frac{1}{2}-\frac{S_i}{2\sqrt{3}} & \quad \text{otherwise}
\end{cases}
\end{align*}
\end{proof}

We may now state the small batch \signSGD{} theorem.

  \begin{tcolorbox}[boxsep=0pt, arc=0pt,
    boxrule=0.5pt,
 colback=white]
\begin{restatable}[Non-convex convergence rate of small-batch 
\signSGD{}]{theorem}{signSGDsmalltheorem}\label{thm:signSGDsmall}
Run algorithm \ref{alg:signSGD} for $K$ iterations under Assumptions 1 to 3. Further, assume that the stochastic gradient noise distribution is unimodal and symmetric (e.g. Gaussian). Set the learning rate and mini-batch size (independently of step $k$) as
  \begin{equation*}
  \delta_k = \frac{1}{\sqrt{\norm{\vec L}_1K}} \qquad \qquad n_k = 1
  \end{equation*}
  Let $N$ be the cumulative number of stochastic gradient calls up to step $K$, i.e.\  $N = \text{O}(K)$. Let $B_k$ be the set of gradient components at step $k$ with large signal-to-noise ratio $S_i := \frac{|g_{k,i}|}{\sigma_i}$, i.e. $B_k := \left\{ i \middle| S_i > \frac{2}{\sqrt{3}} \right\}$. Then we have
  \begin{align*}
  &\mathbb{E}\sq*{\min_{0\leq k \leq K-1} \sq*{ \sum_{i\in B_k} |g_{k,i}| + \sum_{i\not\in B_k} \frac{g_{k,i}^2}{\sigma_i}} } \\
  & \qquad \qquad \qquad \leq \sqrt{\frac{3\norm{\vec L}_1}{N}}\sq*{f_0 - f_* + \frac{1}{2}}
  \end{align*}
\end{restatable}
\end{tcolorbox}

Before we provide the proof, let us make some remarks.

\textbf{Remark 1:} the small batch algorithm achieves the typical $\frac{1}{\sqrt{N}}$ rate.

\textbf{Remark 2:} curiously, the gradient appears in the bound as a \emph{mixed norm}. Large signal-to-noise components see $\ell_1$ convergence barely noticing the noise (except for the worse constant factor compared to the large batch case), and small signal-to-noise components see $\ell_2$ convergence. The transition occurs because as the signal-to-noise ratio shrinks, so does the quality of the sign estimate.

\textbf{Remark 3:} as in the large batch case, there is no explicit dimension dependence in the bound. Again this suggests that depending on the relative geometries of various quantities like gradients, noise and curvature, the algorithm can either converge faster or slower than \SGD{}.

Let's briefly consider the example of sparse noise discussed in the main text for the large batch case. In the small batch bound, all the noise free components will enjoy the fast $\ell_1$ convergence unsullied by the sparse noise. This suggests that small batch \signSGD{} should also perform well in situations with sparse noise.

\textbf{Remark 4:} provided the signal-to-noise ratio of all components shrinks at roughly the same rate, we can expect the optimisation to go through two \emph{phases}. In the first phase, at high signal-to-noise, convergence is $\ell_1$:
  \begin{align*}
  &\mathbb{E}\sq*{\min_{0\leq k \leq K-1} \norm{g_k}_1} \leq \sqrt{\frac{3\norm{\vec L}_1}{N}}\sq*{f_0 - f_* + \frac{1}{2}}
  \end{align*}
whereas in the second phase, at low signal-to-noise, convergence is $\ell_2$:
  \begin{align*}
  &\mathbb{E}\sq*{\min_{0\leq k \leq K-1} \norm{g_k}_2^2 } \leq \norm{\vec \sigma}_\infty \sqrt{\frac{3\norm{\vec L}_1}{N}}\sq*{f_0 - f_* + \frac{1}{2}}
  \end{align*}
The manner in which the noise appears, multiplying the entire right hand side of the bound, is unusual. Also the noise appears linearly rather than quadratically as it does for \SGD{} and large batch \signSGD{}. Perhaps the different modulation of the noise explains the different generalisation properties of solutions found by small-batch \signSGD{}.

Without further ado, here is the proof of Theorem \ref{thm:signSGDsmall}.
\begin{proof}
Following the initial steps taken in proving Theorem \ref{thm:signSGD}, we arrive at
  \begin{align*}
  \mathbb{E}\sq{f_{k+1}-f_k|x_k} &\leq - \delta_k \norm{g_k}_1 +\frac{\delta_k^2}{2}\|\vec L\|_1 \\
  & + 2 \delta_k \sum_{i=1}^d |g_{k,i}|\, \mathbb{P}\sq{\text{sign}(\tilde{g}_{k,i}) \neq \text{sign}(g_{k,i})}
  \end{align*}
By the additional assumption of unimodal symmetric gradient noise, we obtain the tighter bound on failure probability supplied by Lemma \ref{lem:symm}:
\begin{align*}
\mathbb{P}[\text{sign}(\tilde{g}_i)\neq\text{sign}(g_i)] 
&\leq \begin{cases}
\frac{2}{9}\frac{1}{S_i^2} & \quad \text{if } S_i > \frac{2}{\sqrt{3}},\\
\frac{1}{2}-\frac{S_i}{2\sqrt{3}} & \quad \text{otherwise}
\end{cases}\\
&\leq \begin{cases}
\frac{1}{6} & \quad \text{if } S_i > \frac{2}{\sqrt{3}},\\
\frac{1}{2}-\frac{S_i}{2\sqrt{3}} & \quad \text{otherwise}
\end{cases}
\end{align*}
Substituting this in, we get that
  \begin{align*}
  &\mathbb{E}\sq{f_{k+1}-f_k|x_k} \\
  &\leq - \delta_k \norm{g_k}_1 +\frac{\delta_k^2}{2}\|\vec L\|_1 + 2 \delta_k \sum_{i\in B_k} \frac{|g_{k,i}|}{6}\\ &+ 2 \delta_k \sum_{i\not\in B_k} |g_{k,i}|\left[\frac{1}{2}-\frac{|g_{k,i}|}{2\sqrt{3}\sigma_i}\right]\\
  &= - \delta_k \sum_{i=1}^d |g_{k,i}|+\frac{\delta_k^2}{2}\|\vec L\|_1 + \delta_k \sum_{i\in B_k} \frac{|g_{k,i}|}{3}\\ &+ \delta_k \sum_{i\not\in B_k} |g_{k,i}|- \delta_k \sum_{i\not\in B_k} \frac{g_{k,i}^2}{\sqrt{3}\sigma_i}\\
    &= - \frac{2\delta_k}{3} \sum_{i\in B_k} |g_{k,i}| - \delta_k \sum_{i\not\in B_k} \frac{g_{k,i}^2}{\sqrt{3}\sigma_i}+\frac{\delta_k^2}{2}\|\vec L\|_1
  \end{align*}
  Interestingly a mixture between an $\ell_1$ and a variance weighted $\ell_2$ norm has appeared.
  Now substitute in the learning rate schedule, and we get:
    \begin{align*}
  &\mathbb{E}\sq{f_{k+1}-f_k|x_k} \\
    &\leq - \frac{2}{3\sqrt{\norm{\vec L}_1K}} \sum_{i\in B_k} |g_{k,i}| - \frac{1}{\sqrt{3\norm{\vec L}_1K}} \sum_{i\not\in B_k} \frac{g_{k,i}^2}{\sigma_i}+\frac{1}{2K}\\
&\leq - \frac{1}{\sqrt{3\norm{\vec L}_1K}} \sq*{\sum_{i\in B_k} |g_{k,i}| - \sum_{i\not\in B_k} \frac{g_{k,i}^2}{\sigma_i}}+\frac{1}{2K}
  \end{align*}
  Now telescope over the iterations:
    \begin{align*}
    &f_0 - f^* \\
    &\geq f_0 - \mathbb{E}\sq{f_K} \\
    &= \mathbb{E}\sq*{\sum_{k=0}^{K-1}f_k - f_{k+1}} \\
    &\geq \frac{1}{\sqrt{3\norm{\vec L}_1 K}}\mathbb{E}\sum_{k=0}^{K-1}\sq*{\sum_{i\in B_k} |g_{k,i}| + \sum_{i\not\in B_k} \frac{g_{k,i}^2}{\sigma_i} } - \frac{1}{2}\\
    &\geq \sqrt{\frac{K}{3 \norm{\vec L}_1}}\mathbb{E}\sq*{\min_{0\leq k \leq K-1} \sq*{ \sum_{i\in B_k} |g_{k,i}| + \sum_{i\not\in B_k} \frac{g_{k,i}^2}{\sigma_i}} } - \frac{1}{2}
  \end{align*}
  Finally, rearrange and substitute in $N = K$ to yield the bound
  \begin{align*}
  &\mathbb{E}\sq*{\min_{0\leq k \leq K-1} \sq*{ \sum_{i\in B_k} |g_{k,i}| + \sum_{i\not\in B_k} \frac{g_{k,i}^2}{\sigma_i}} } \\
  & \qquad \qquad \qquad \leq \sqrt{\frac{3 \norm{\vec L}_1}{N}}\sq*{f_0 - f_* + \frac{1}{2}}
  \end{align*}
  
\end{proof}
